# Supplementary material for: DreaMontage: Arbitrary Frame-Guided One-Shot Video Generation
Source: arXiv:2512.21252 source file (2025-12-25)
Supplement: Supplementary file 1 [file Appendix.tex]

\appendix
\section*{Contributions and Acknowledgments}

% \noindent
% All contributors of DreaMontage are listed below.

% \vspace{1em}

% \noindent
% % 直接横向排列，自动换行
% Jiawei Liu$^*$, Junqiao Li$^*$, Jiangfan Deng$^*$, Gen Li, Siyu Zhou, Zetao Fang, Shanshan Lao, Zengde Deng, Tingting Ma, Jianing Zhu, Jiayi Li, Yunqiu Wang, Qian He, Xinglong Wu.

% \vspace{2em}
% \noindent{$^*$ Equal contributions.}

\noindent
All contributors of DreaMontage are listed below.

\vspace{1em}

\noindent
\begin{minipage}[t]{0.48\textwidth}
    \textbf{\large Core Contributors}
    \vspace{0.5em}
    
    Jiawei Liu$^*$ \\
    Jiangfan Deng$^*$ \\
    Junqiao Li$^*$ \\
    Gen Li \\
    Siyu Zhou \\
    Zetao Fang \\
    Qian He \\
\end{minipage}%
\hfill
\begin{minipage}[t]{0.48\textwidth}
    \textbf{\large Contributors}
    \vspace{0.5em}
    
    Shanshan Lao \\
    Zengde Deng \\
    Tingting Ma \\
    Jianing Zhu \\
    Jiayi Li \\
    Yunqiu Wang \\
    Xinglong Wu
\end{minipage}

\vspace{2em}
\noindent{$^*$ Equal Contribution.}
